# Supplementary material for: Imitating Interactive Intelligence
Source: arXiv:2012.05672 source file (2021-01-21)
Supplement: Supplementary file 1 [file example_human_instructions.pdf]

# Examples of instructions and responses from human demonstrations

For each combination of prompt and modifier we show 10 examples of setter instructions and, where applicable, the solver's response. The setter's instruction is shown in blue, and the solver's response in orange. "..." is used to denote multiple utterances.

## Ask the other player to count something

### No modifier

"Count number of objects in the room." → "21"  
"Count the items on the bed?" → "two"  
"count the objects on the floor" → "10"  
"count balls" → "Two, 2."  
"count the objects on the bed" → "three"  
"how many balls are there?" → "five"  
"count all the objects" → "13"  
"count the objects which is on floor" → "13"  
"count the balls" → "Five"  
"count objects in the room." → "15"

### Try to refer to objects by colour

"count the white rectangular objects" → "Three"  
"Count the no of pink objects." → "9"  
"How many red color objects are there?" → "five."  
"count the number of gray objects in the room?" → "one"  
"count the number of red color objects." → "three"  
"count orange color objects." → "Six"  
"count number of white objects" → "one"  
"Count pink objects" → "7"  
"count objects on floor" → "17"  
"count red color object" → "five."

### Try to refer to objects by location

"count all the objects on the floor" → "11"  
"count objects on the table" → "one"  
"count the objects which are on the floor?" → "13"  
"count the objects on the floor" → "10"  
"count the objects which are on floor" → "12"  
"count the objects on floor but only pillows" → "five"  
"Count objects on the bed." → "four"  
"count the objects on the floor" → "12"

"Count the objects which are not on bed" → "12"  
"count the objects which are on the teal color table" → "Two"

Try to use words like: not, isn't

"count the objects which are not on the floor" → "7"  
"count of objects not on the floor?" → "7"  
"count objects which are not on floor" → "four"  
"count objects which are not red." → "10"  
"count the toys which are not on the table?" → "10"  
"count the objects which are not on floor?" → "Seven"  
"count number of objects which are not on the floor" → "8"  
"count the objects which are not on the floor" → "8"  
"count objects which are not in yellow" → "nine"  
"count the objects which are not on the bed" → "16"

Try to use shape words like: circular, rectangular, round, pointy, long

"count the circular objects" → "one."  
"count the pointy objects" → "two"  
"Count the number of rectangular objects." → "Two"  
"get me a count of the rectangular pianos?" → "two."  
"get me a count of the pointy rockets?" → "one"  
"count the number of circular objects in the room" → "2 objects"  
"count the rectangular objects" → "7"  
"count the pointy objects in the room" → "three."  
"count the round objects" → "0"  
"count rectangular objects in room" → "three"

## Ask the other player to describe where something is

No modifier

"where is the red ball" → "on the floor"  
"Where is the Pink Duck?" → "on the shelf"  
"where is the green cupboard" → "Near magenta color chair at near one corner of the room"  
"Where is green lamp?" → "Near the bed."  
"where is red ball?" → "It is on the shelf."  
"Describe where is the white book?" → "bed"  
"Describe the blue photo frame where it is" → "on floor next to the yellow table"  
"Where is the green color lamp?" → "on bed"  
"where is the red teddy placed" → "near to the door"  
"where is the cactus located" → "on the table"

Try to refer to objects by colour

"where is the purple color ball?" → "bed"

"describe where is white ball" → "on the bed"  
"Where is pink rocket?" → "on the bed"  
"Where is the red colored mug in the room ?" → "On the blue table"  
"describe where is sea green duck?" → "on the floor"  
"where is the blue rocket" → "Close to the Door"  
"where is green rectangular table?" → "On the floor."  
"Where is the cyan duck?" → "on the bed"  
"Where is the orange colored cupboard exist in the room ?" → "beside bed on the floor"  
"Where is red robot?" → "On the bed."

Try to use words like: not, isn't

"Where is plane which is not in orange color." → "on the floor"  
"Where is the ball which is not on the bed?" → "next to violet cup"  
"where is the other pot which is not on the floor" → "on the bed"  
"where is green duck which is not on floor" → "on bed"  
"where is mirror which isn't on the floor?" → "On the rack."  
"Where is rocket placed which is not on floor" → "on the wooden shelf"  
"Where is red hair drier which is not on the floor?" → "on the bed"  
"where is the pillow which is not on the table" → "on the floor"  
"where is the pointy object which is not on shelf?" → "on bed"  
"describe where the hairdryer is which is not on the bed" → "On the table"

Try to use shape words like: circular, rectangular, round, pointy, long

"where is the pink circular object?" → "on bed"  
"Describe where white color circular object is?" → "Near the blue chair."  
"Describe where is the rectangular object." → "on the floor near the white box"  
"Where is the circular object in the room" → "on the bed."  
"Where is green rectangular object" → "On the floor"  
"where is the round object?" → "on the floor"  
"where is the circular ball present" → "On the bed"  
"where's the rectangular green book?" → "on the floor"  
"where are the rectangular pink objects?" → "on the bed"  
"where is the rectangular book?" → "On the bed"

Ask the other player to do something, then when they are finished, ask them to do something else

"keep the pink ball on bed... now count objects on floor" → "6"  
"lift the plane... put the lamp on the bed"  
"put pink ball in the pink basket... and now count the items on the bed." → "3"  
"Go near to the window... What could you see through the window?" → "Nothing"  
"clear pink table. count the number of objects on bed" → "4"  
"put the green mug on the sofa... count the mugs in the room." → "5"  
"Lift the yellow color lamp... Put white color ball on the shelf"

"put two ash pillows on the bed... put white ball in purple box"  
"keep piano on book and wait.. keep train on bed"  
"place three orange objects in a row... count number of green objects." → "Three"

## Ask the other player to perform an activity of your choice

"keep 5 objects in a circle"  
"put all blue items in a line"  
"What could you observe through the window?" → "it has a mirror. i can objects from far"  
"grab orange gadget and roam around the room"  
"bring me a piano"  
"stand on bed and do whatever u want to do" → "done"  
"Put the red cup on the sofa as shown in the room" → "yes"  
"count items in the room" → "eleven"  
"perform an activity of your choice"  
"Lift pink ball."

## Ask the other player to go somewhere

### No modifier

"go near the door?"  
"go near to the bed"  
"Go near the pink chair"  
"Go and stand at any corner of the room."  
"Go near the red table."  
"Go near the white table."  
"Go near the door."  
"Go and stand near the door."  
"go left to the sea green color cupboard" → "No I can't"  
"go close to white rack"

### Do not use the words: bed, door, window

"go near the chair"  
"go near red box"  
"go near sofa"  
"go near the pink table"  
"go to any wooden shelf"  
"Go near the white cupboard"  
"go near the pink table."  
"go near the red basket"  
"go to blue color racket." → "it's not blue. purple"  
"go near an orange color basket"

Try to refer to the location by colour

"go and stand in front of the white door"  
"go near the blue bookcase"  
"go close to the red bed"  
"stand near green bin"  
"go near white color book"  
"go near the violet colored storage box"  
"go to blue chest"  
"stand next to green box"  
"go near the pink cupboard"  
"go and stand in front of the blue color lamp"

Try to use words like: in front, behind, left of, right of, between

"stand left to door"  
"go left of yellow wardrobe"  
"stand near orange color storage box"  
"Go behind pink basket"  
"stand in front of closet"  
"go between sofa and bin"  
"go and stand in front of the window"  
"stand in between the two tables"  
"go in front of a bed"  
"go in front of the window"

Try to use words like: near, far, close to, next to

"go near to the bed"  
"go near to car which is close to mug"  
"go near the door"  
"go near the door"  
"Go close to the door."  
"go next to a bed"  
"go near to door"  
"Go near the table."  
"Go near the blue table"  
"go near to the door"

## Ask the other player to lift something

No modifier

"lift green ball from bed"  
"Lift any object."  
"lift the basket ball on the bed"  
"Lift the bed." → "impossible"  
"lift the pink dryer that is on the floor" → "No pink dryer on floor"

"pick the orange colour ball"  
"lift purple table"  
"Lift the red color chair."  
"lift the orange boat"  
"lift blue color book on floor"

#### Try to refer to objects by colour

"lift pink color chair"  
"lift blue bin"  
"lift the red color piano"  
"lift the white lamp"  
"lift the violet teddy."  
"lift orange colour robo"  
"lift the blue color frame"  
"lift pink ball which is on the floor"  
"Lift white color rocket."  
"lift a cyan object on the bed"

#### Try to refer to objects by location

"lift the ball which is near to orange color bed"  
"Lift the violet colored rectangular shaped object off the bed."  
"Lift the red color robot which is on the floor."  
"lift the grey color pillow near to the violet color chair"  
"lift the mug which is on the bed"  
"lift the circular ball on the bed"  
"Lift the ball on the bed"  
"lift the robot which is on the shelf"  
"lift the mug from the bed"  
"lift the teddy which is on the bed"

#### Try to use words like: in front, behind, left of, right of, between

"lift the pillow left of the bed"  
"lift the keyboard in front of the red robot"  
"lift the photo frame placed in front of the green chair"  
"lift the frame in front of the table"  
"lift the stool which is left of violet rack"  
"Lift the stool which is left to the door."  
"lift the green chair in front of the orange cup board"  
"Lift the boat which is in front of the bed"  
"lift the racket which is in front of the bed"  
"lift the carriage which is in front of the bed"

#### Try to use words like: not, isn't

"lift the book which isn't on the pink table"  
"Lift anything which isn't present on the bed."

"lift the keyboard which is not in red color"  
"identify the color of plane which is not on the bed."  
"lift mug which is not on floor"  
"Lift potted plant which is not on the floor"  
"Lift ball, which is not on floor."  
"lift up the stool which is not in the blue color"  
"lift the object which is not on bed and floor"  
"lift the rocket which is not on bed"

Try to use words like: near, far, close to, next to

"lift the pink hair dryer which is near the door"  
"lift a box close to the table"  
"lift the book which is close to the red chair"  
"lift the ball which is near the bed?"  
"Lift the duck near the sofa?"  
"Lift a robot, which is near the bed."  
"Lift the sofa which is near to the bed."  
"lift the duck which is close to the table"  
"lift up the pot which is close to the bed"  
"Lift the mug near the bed."

Try to use shape words like: circular, rectangular, round, pointy, long

"lift any rectangular shape object."  
"lift the pointy object which is on the bed" → "boat is not a pointy object"  
"lift round ball from the bed"  
"lift circular object in the room"  
"lift one pointy object"  
"lift the rectangular book from the table"  
"Lift any round object"  
"Lift the circular ball."  
"lift circular ball"  
"lift something pointy"

Try to use words like: on top, beneath, above, below

"lift teddy which is on top of the bed"  
"Lift the boat on top of yellow table"  
"Lift the object from the yellow table"  
"Lift orange color rubber duck that is on top of the bed"  
"lift the cyan color ball which is on top of blue table"  
"lift the pot which is on top of bed"  
"lift the racket which is above the bed"  
"Lift the mug from top of the table"  
"lift any object which is on top of bed"  
"lift a ship which is on white color table"

Ask the other player to put three or more specific objects in a row

"place 4 objects in row"  
"put all the balls in the row"  
"Put the objects on the bed in a row."  
"Place any six objects in a row"  
"arrange balls in a row"  
"put the violet things in a row"  
"put 5 objects in a row"  
"put any three objects in a straight line"  
"keep all the green objects in a row"  
"place any 3 objects in a row"

Ask the other player to position something relative to something else

No modifier

"Place the green teddy near the pink mug"  
"Put the pink mug on the pink table."  
"place the red chair beside the violet sofa?"  
"Put the mug on the bed"  
"keep the mirror under the table"  
"put the pink hair dryer on the bed"  
"Place the red robot in the box... pink box."  
"place the pink duck on the floor"  
"place pink mirror in red box"  
"place white in the white box?... white ball"

Try to refer to objects by colour

"Place the white lamp on the bed."  
"Place the white color plane in front of bed"  
"put the orange pot near the red stool"  
"Pick yellow robot and place it in the grey sofa"  
"place the orange box near to the yellow table"  
"place the pink box on bed"  
"place the green ball in the basket"  
"place any violet object in violet box"  
"place the green mug on the table."  
"Position the cyan pot near any orange object"

Try to refer to objects by location

"Place the pillow which is in the corner of the room in the basket."  
"put the box on the bed"  
"Place white rubber duck on top of the table?"  
"place the red ball in the basket which is on the table."



"place the orange chair near the bed"  
"take the purple color plant from the table and keep it on the bed"  
"place yellow lamp next to cactus plant"  
"Place the yellow mirror on bed which is on top of table."  
"place green duck near green chair"  
"Put the basketball inside the box."

Try to use words like: in front, behind, left of, right of, between

"place the blue mug in front to the bed"  
"Place the orange color duck right in front of the door"  
"place red duck in front of bed"  
"place a pink basket in front of pink ball"  
"put the any object on the bed"  
"place orange mug in front of green ball"  
"place a orange piano beside the bed."  
"place pink piano in front of pink boat"  
"place orange mug in front of green ball"  
"place the red plane in front of the bed"

Try to use words like: not, isn't

"place yellow drier which is not on floor on table"  
"Place the red color mirror in front of the door, you are able to see one red color mirror on the floor, isn't?" → "yes"  
"Put duck on the bed which is not in white color."  
"place the mirror in the basket which is not on the bed"  
"place the car near the door which isn't on the floor"  
"place ash color object which is not on bed on pink chest"  
"Place ball on bed but not on floor"  
"place keyboard which is not present on floor on bed"  
"place the teddy bear which is not green color on the bed"  
"place the lamp on the book which is not on the floor"

Try to use words like: near, far, close to, next to

"place the white ball close to the bed"  
"Put two pots next to each other."  
"keep the yellow pot far from the table"  
"put the keyboard far from the bed"  
"place the chair near the bed."  
"place the red pillow near to white duck"  
"Place basket next to the chair."  
"keep the pink mug near to another pink mug"  
"Place red color potted plant near to the bed"  
"place orange color robot near the bed."

Try to use shape words like: circular, rectangular, round, pointy, long

"place round ball on cyan table"  
"place the rectangular mirror near the door."  
"place the pink circular object on the floor"  
"place the rectangular piano on bed"  
"place violet rectangular object on bed"  
"place the circular ball in front the door"  
"place the circular object near the door."  
"Place the circular stool in the rectangular basket"  
"place the pointy object on the bed"  
"put the circular ball on the bed."

Ask the other player to stand in some position relative to you

"stand in front of me"  
"stand in front of me?"  
"Stand right in front of me."  
"stand on my right"  
"stand in front me"  
"Stand in front of me."  
"stand opposite to me"  
"stand near to me"  
"stand beside me."  
"stand next to me"

Ask the other player to push an object around using another object

"Push the sofa with some object"  
"push the orange plane using green plane"  
"push sofa with pillow"  
"push the ball using ball"  
"push the chair using ball"  
"Push white mirror with the purple teddy."  
"Push the white box with green mug"  
"push the duck using the bus"  
"push the orange duck using the keyboard"  
"push any green object using an other green object"

Ask the other player to put something on top of something else

"put the yellow ball on white table"  
"Place the teddy top of the pink rack."  
"place a stool on bed"  
"place the pink duck on top of the bed"

"Put yellow duck on stool."  
"Place the pink duck on white table"  
"Place the white piano on the top of orange coloured book" → "yes"  
"put the yellow duck on top of the green box"  
"place green headphones on top of the table?"  
"Place the olive green colored cushion on top of the pink table."

## Ask the other player to put something underneath something else

"Place orange color racket under green color chair."  
"put something underneath something else"  
"place the green lamp under the shelf"  
"put pink rocket under the orange table"  
"Place blue headphones under the yellow table"  
"Place hair dryer under the table... sorry shelf"  
"place the helicopter under the chair"  
"Put green color boat underneath table"  
"Put green book under the green table"  
"put the teddy under the table"

## Ask a question about the color of something

### No prompt

"color of floor" → "brown"  
"colour of ball on pink book" → "Blue"  
"color of the book on the bed" → "white"  
"color of roof?" → "Pale pink"  
"color of the roof?" → "green"  
"color of helicopter on bed" → "dark green"  
"what is the color of pillow on the floor" → "purple red"  
"what is the color of box" → "orange"  
"Color of the teddy on the bed?" → "Red"  
"what is the color of bed" → "yellow"

### Try to refer to objects by location

"Color of teddy on bed" → "brown"  
"Color of dryer from bed" → "orange"  
"Color of bus on bed ?" → "grey"  
"color of keyboard which is on the table?" → "blue"  
"color of objects at corner of room" → "yellow"  
"colour of mug on bed" → "yellow"  
"Tell me the color of a rack which is near to the window" → "pink"  
"what are the colors of the teddys on the bed?" → "green and violet"  
"what is the color of basket in the room" → "pink"  
"color of the stool near the window" → "Purple."

Try to use words like: in front, behind, left of, right of, between

"color of the lamp to the left of bed" → "pink"  
"color of the boat which is in front to the blue stool" → "white"  
"what is the color of the cup in front of the cupboard" → "red"  
"color of book in front of bed" → "white"  
"What is the color of ball which is left to the bed ?" → "orange"  
"colour of box in front of violet table?" → "yellow"  
"color of the mug in front of the orange rocket" → "red"  
"what is the color of the boat which is in between blue ball and red table?" → "pink"  
"color of plane in front of bed" → "pink"  
"what is the color of pillow in front of the cupboard.?" → "brown"

Try to use words like: not, isn't

"color of drier which is not on floor" → "violet"  
"what is the color of storage box which is not yellow?" → "blue"  
"Color of the robot which is not on the floor" → "yellow."  
"color of teddy which is not on bed?" → "green, violet"  
"color of the frame which is not on the floor" → "orange"  
"What is the color of the robot which is not in pink" → "sea green color"  
"Color of the keyboard which is not on floor" → "white"  
"what is the color of the ball which is not on the bed" → "purple and blue."

Try to use words like: near, far, close to, next to

"What's the color of the ball that's on top of the orange table?" → "sea green"  
"Color of robot near the bed" → "pink"  
"color of the robot close to the box." → "cyan"  
"what is the color of the robot which is near the bed" → "sea green"  
"color of the robot which is near to the pink chair" → "pink"  
"Colour of the basket close to the door?" → "magenta"  
"color of the table near the bed" → "white"  
"color of pot near bed" → "white color"  
"color of bin close to pink table?" → "purple"  
"what is the color of the duck which is near the cupboard?" → "sea green"

Try to use words like: some, all, most, many, none

"Can you tell me the color of tables in the room?" → "yellow and green"  
"color of all objects on bed" → "yellow"  
"Color of all objects on the bed." → "white"  
"color of none of the objects in the room" → "Black"  
"color which is mostly visible in the room" → "purple"  
"what is the color of most of the objects?" → "blue"  
"what is the color of the bed?" → "Violet"  
"what is the color of objects which are most on the bed" → "green"  
"What is the color that none of the objects are having" → "Green"  
"color of most of the objects in the room" → "orange"

Try to use shape words like: circular, rectangular, round, pointy, long

"color of rectangular door" → "White"  
"Color of the circular object which is on the bed" → "pink and green"  
"what is the colour of rectangular carriage which is on bed" → "purple"  
"what is the color of circular object that is on the bed?" → "pink"  
"What is the color of ball which is on the yellow color table" → "Cyan color."  
"color of ball near the bed" → "cyan"  
"Colour of long table?" → "blue"  
"what is the colour of circular object on bed" → "light pink"  
"color of circular object on floor" → "red and orange"  
"color of rectangular object on bed" → "purple"

Try to use words like: on top, beneath, above, below

"color of teddy on top of the bed" → "purple"  
"what is the color of the ball on top of the bed?" → "Green"  
"what is the color of a ball, which is on the bed." → "Pink."  
"what is the color of boat which is on top of light pink table" → "white"  
"what is the color of the bus on the white table" → "mauve"  
"color of the bats which is on the green table" → "pink"  
"color of the carriage on the top of the bed?" → "violet"  
"color of bus on table" → "lite pink"  
"Color of lamp which is on top of bed" → "sea green"  
"what is the color of the object which is on the bed" → "green"

Ask the other player whether a particular thing exists in the room

"any pillow exist in the room" → "no"  
"Do we have books in room ?" → "No"  
"Is there a green color sofa?" → "Yes."  
"is there any bike in this room?" → "no"  
"Do we have Red ball in the Room?" → "Yes"  
"is there a red helicopter in this room?" → "Yes"  
"Whether there is a book in the room?" → "no"  
"Green color bat is there in the room" → "yes"  
"does any red color bed exist in the room?" → "no"  
"is the red lamp exists in room" → "yes"

Ask the other player to say what they are looking at or noticing right now

"what you are noticing right now?" → "red basket"  
"what are you looking right now" → "you"  
"what are you looking right now" → "orange pot"  
"what are you looking at" → "looking at the objects on the orange table"  
"What are you looking right now?" → "The red colored football that's on the floor."

"what u r noticing right now" → "a blue mug"  
"what are you looking at?" → "Blue lamp on the floor."  
"What are you noticing right now?" → "bed"  
"what are you looking at?" → "Things on the bed."  
"what are you looking at?" → "floor"

## Ask the other player to touch an object using another object

"touch bed using red basket"  
"touch green headphones with other green headphones"  
"touch white boat with blue robot"  
"touch pink colour book using purple colour which is on the floor"  
"touch the table with rocket"  
"touch the white ball by using the blue piano"  
"touch the orange robot by using white box"  
"touch the toy car using any other object"  
"touch yellow book using blue book"  
"Touch the red rocket with the yellow football which is on the floor."
