# Supplementary material for: Imitating Interactive Intelligence
Source: arXiv:2012.05672 source file (2021-01-21)
Supplement: Supplementary file 2 [file example_language_games_instructions.pdf]

# Instructions for Language Games with Modifiers (2-player)

[Overall procedure](#)

[Instructions for Setters](#)

[Advice for giving good instructions](#)

[Instructions for Solvers](#)

[Game scripts](#)

- [1. Ask the other player to position something relative to something else.](#)
- [2. Ask a question about the color of something.](#)
- [3. Ask the other player to lift something.](#)
- [4: Ask the other player to go somewhere.](#)
- [5: Ask the other player to count something.](#)
- [6: Ask the other player to describe where something is.](#)

## Overall procedure

- Each day, raters should be split into two groups of equal size: A and B.
- The two groups should be seated apart from one another in order to ensure that they can't see each other's screens, or communicate outside of the chat box.
- Pairs should be randomly chosen, one person from group A and one from group B.
- Group A will start out by playing as Setters, and group B will start by playing as Solvers.
- After playing together for 30 minutes the players should swap roles within their pairs, so that the player from group B becomes the Setter and the player from group A becomes the Solver.
- After playing together for another 30 minutes the pairs should be randomly shuffled, so that each player from group A is paired with a different partner from group B.
- Group A will then become the Setters again, and group B will play as Solvers.
- This cycle should continue, with players switching roles within their pairs every 30 minutes, and swapping partners every hour.

# Instructions for Setters

1. **Enter the game and send the link to the other player.** Follow this link - you should see a pop-up menu titled “**New game: Language Games with Modifiers (2 Player)**”. Click on the button in the bottom right corner that says “**Go**”. You will see two links pop up. Copy the second link and send it to your paired rater. Then click on the “**Play**” button next to the first link.
2. **Read the game script and think of an instruction.** You will be placed in a room with another player and a number of objects. At the top of the screen you will see a [game script](#), which indicates your objective in this game. Start out by moving around the room to see what objects are present. Then, following the game script, think of an instruction for the other player to carry out. Make sure that what you’re asking them to do is actually possible. For example, don’t ask the other player to “Pick up a teddy bear” if there are no teddy bears in the room!
3. **Send your instruction to the other player.** Use the enter key to switch between gameplay and typing your instruction. Once you have written the instruction, hit Enter again to send it to the other player. You must only send one instruction, so type carefully! Messages between players will show in the 'chat' area above where text is typed.
4. **Watch and check that the other player follows your instruction.** Move around the room to get a good view of what the other player is doing.
5. **End the episode.** If the other player completes the instruction or if you are sure they will not be able to complete your instruction correctly, end the episode by pressing the "6" key. If you don't press the “6” key then the episode will end automatically after two minutes. Please end the episode immediately when the task is completed - you should only send one instruction per episode.
6. **Give scores for yourself and the other player.** After the episode ends you will be asked to give scores for how well you think both you and the other player performed the game. Type your answers into the text box. These scores are anonymous and won't be used to rate your performance in any way, so please answer honestly.
7. **End the game if you are finished or need a break.** When you have finished playing all episodes or are taking a break, please delete the game by clicking the bin icon on the lower right hand side of the page.

## Advice for giving good instructions

- **Read our examples.** We have provided some examples of good instructions for each [game script](#). These are only intended as a guide - the room will be different for every episode, so you will need to adapt your instructions to the specific room you are in.
- **Be creative.** For example, there are often many different ways you could refer to the objects in the room, or to say the action you would like the other player to carry out. If you can, **try to use a different instruction each time** in order to keep things interesting for you and the other player!
- **Use simple English.** Instructions should be clear and understandable to the other player, and they should only refer to things that are in the room.

- **Use full sentences.** For example, “*How many boxes are there?*” and “*Count the number of boxes.*” are both examples of good instructions for [script 5](#), however “*Number of boxes*” is not a good instruction because it isn’t a complete sentence.

## Instructions for Solvers

1. **Follow the link sent by the other player to enter the game.** If it works, you should both see a loading page and then after some delay the game will begin. You will be placed in a room with another player and a number of objects.
2. **Wait for an instruction sent by the other player.** After some time the other player in the room will give you an instruction telling you what to do. Messages between players will show in the 'chat' area above where text is typed. While waiting for the instruction, feel free to move around the room to get familiar with the various objects and their layout.
3. **Follow the instruction.** Once you receive the instruction, try to follow it to the best of your abilities. If the instruction requires you to send a message back to the other player, change from 'moving' to 'typing' mode by pressing Enter, type your response, and then hit Enter again to send it. Please only send one response per instruction.
4. **Wait for the other player to end the episode.** The episode will end when the other player thinks you have completed the game, or after a time limit of two minutes.
5. **Review the performance of you and the other player.** After the other player terminates the game you will be asked to give scores for how well you think both you and the other player performed the game. Type your answers into the text box. These scores are anonymous and won't be used to rate your performance in any way, so please answer honestly.
6. **End the game if you are finished or need a break.** When you have finished playing all episodes or are taking a break, please delete the game by clicking the bin icon on the lower right hand side of the page.

# Game scripts

At the start of each episode the Setter will see a game script consisting of an **instruction type** and, in most cases, a **modifier**. The instruction type tells the setter what kind of instruction they should give to the solver. The modifier contains additional requirements that the setter's instruction should satisfy.

For example:

**Ask the other player to position something relative to something else. Try to refer to objects by their colors.**

Some examples of good instructions for this game script are:

*Put a blue thing next to the red thing on the bed*  
*Place a green toy on the shelf by the door*  
*Put the orange duck next to the magenta one*

The following examples are not as good:

*Put a robot next to the lamp*  
*Place a book on the table*  
*Take the toy from the bed and put it on a shelf*

Even though they are the right overall type of instruction, none of them refer to objects by their color, so they don't satisfy the requirement in the modifier.

Sometimes the game script will just contain the instruction type without any modifier, for example:

**Ask the other player to position something relative to something else.**

In these cases the Setter can give any instruction as long as it's of the correct type.

The full list of instruction types and modifiers are given below.

## 1. Ask the other player to position something relative to something else.

- Try to refer to objects by color.
- Try to refer to objects by location.
- Try to use shape words like: circular, rectangular, round, pointy, long.
- Try to use words like: near, far, close to, next to.
- Try to use words like: in front, behind, next to, left of, right of.
- Try to use words like: not, isn't.

## 2. Ask a question about the color of something.

- Try to refer to objects by location.
- Try to use shape words like: circular, rectangular, round, pointy, long.
- Try to use words like: near, far, close to, next to.
- Try to use words like: in front, behind, next to, left of, right of.
- Try to use words like: on top, beneath, above, below.
- Try to use words like: some, all, most, many, none.
- Try to use words like: not, isn't.

## 3. Ask the other player to lift something.

- Try to refer to objects by color.
- Try to refer to objects by location.
- Try to use shape words like: circular, rectangular, round, pointy, long.
- Try to use words like: near, far, close to, next to.
- Try to use words like: in front, behind, next to, left of, right of.
- Try to use words like: on top, beneath, above, below.
- Try to use words like: not, isn't.

## 4. Ask the other player to go somewhere.

- Try to refer to the location by color.
- Try to use words like: near, far, close to, next to.
- Try to use words like: in front, behind, next to, left of, right of.
- Do not use the words: bed, door, window.

## 5. Ask the other player to count something.

- Try to refer to objects by color.
- Try to refer to objects by location.
- Try to use shape words like: circular, rectangular, round, pointy, long.
- Try to use words like: not, isn't.

## 6. Ask the other player to describe where something is.

- Try to refer to objects by color.
- Try to use shape words like: circular, rectangular, round, pointy, long.
- Try to use words like: not, isn't.
